# Supplementary material for: HPSCAN: Human Perception-Based Scattered Data Clustering
Source: arXiv:2304.14185 source file (2025-01-30)
Supplement: Supplementary file 1 [file supplementary.pdf]

*Volume xx (200y), Number z, pp. 1–11*

# Supplementary Material
# HPSCAN: Human Perception-Based Scattered Data Clustering

S. Hartwig[1] C. v. Onzenoodt[1], D. Engel[1], P. Hermosilla[2] and T. Ropinski[1]

[1]Visual Computing Group, Ulm University, Germany
[2]Computer Vision Lab, Technical University of Wien, Austria

## 1. User Interface

Figure 1 displays the user interface for the crowdsource study, where we collected human annotations for clusterings perceived in a scatterplot. Participants are provided with a scatterplot and can select different colors to categorize points into clusters. The brush size for selecting points can be adjusted with a slider or mouse wheel, and participants can add new colors for additional clusters, maximum 20. There is also an option to indicate if no clusters are visible. Once clustering is complete, participants can proceed by clicking 'Continue'. In total, each participant had to annotate 20 scatterplot images. To identify bots or *click-through* behavior, we included three additional sanity checks. These checks display stimuli with multiple spatially separated Gaussian blobs that form visually distinct clusters. One example of such a stimulus, used as a sanity check, has predefined ground truth cluster boundaries as can be seen in Figure 1. If a participant's segmentation deviated by more than 30% from the target measured in IoU, they failed this check. Data from participants who failed more than one sanity check was discarded.

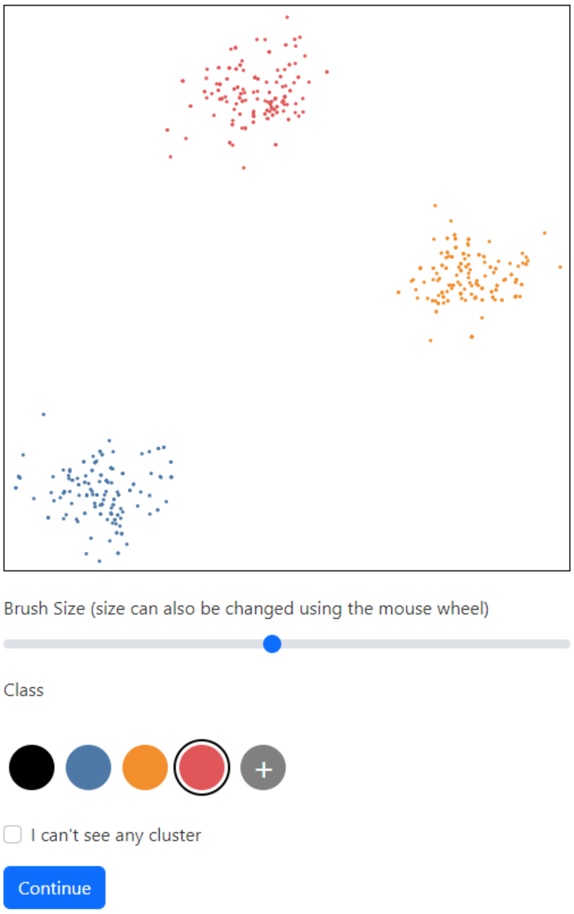


Figure 1: User interface for a crowdsourcing study displaying a sanity check used to detect *click-through* behavior and bots. Participants can adjust the brush size using a slider or the mouse wheel. Colors can be arbitrarily assigned to brush different clusters.

## 2. Contrastive Loss Weighting Analysis

The results in Table 1 illustrate the impact of the weighting factor $D$ on the clustering behavior of HPSCAN. Observing the results for the single cluster column, lower values of $D$ result in a $\kappa_\alpha$ metric that remains relatively high, indicating that clusters are being treated as larger, more cohesive groups. However, as $D$ increases, the $\kappa_\alpha$ metric gradually decreases, reflecting a tendency of the algorithm to identify finer structures within the data, leading to the division of larger clusters into several smaller ones. This trend is evident at $D = 0.1$, where $\kappa_\alpha$ is relatively high; as $D$ increases to values like $D = 50.0$ and $D = 100.0$, the $\kappa_\alpha$ metric decreases significantly, suggesting a more fragmented clustering outcome as the influence of the weighting factor grows. In contrast, when examining results in the five- and six-cluster columns, an opposite trend can be observed.

At the same time, the $\kappa_v$ metric generally increases with $D$, indicating improved consistency in the assignment of these smaller clusters. This trend suggests that HPSCAN becomes more sensitive to subtle distinctions in the data, allowing for more detailed

clustering at higher $D$ values. In summary, increasing $D$ results in a shift from broader clusters to a more granular clustering structure, capturing finer groupings in the data.

Table 1: Detailed results of our Contrastive Loss Weighting Analysis, reporting scores for all cluster numbers individually.

| $D$ | | No Cluster | One Cluster | Two Clusters | Three Clusters | Four Clusters | Five Clusters | Six Clusters | $\Sigma$ |
|---|---|---|---|---|---|---|---|---|---|
| 0.1 | $\kappa_\alpha \uparrow$ | 1.2284 | -0.0247 | -0.3765 | -0.5695 | -1.3971 | -1.7102 | -2.7922 | -5.6418 |
| | $\kappa_v \uparrow$ | 0.2775 | 0.0295 | 0.0333 | 0.0281 | 0.0441 | 0.0563 | 0.0639 | 0.5327 |
| 1.0 | $\kappa_\alpha \uparrow$ | 1.2284 | 0.0027 | -0.4022 | -0.6256 | -1.6394 | -1.7682 | -3.1288 | -6.3330 |
| | $\kappa_v \uparrow$ | 0.2775 | 0.0268 | 0.0202 | 0.0223 | 0.0235 | 0.0351 | 0.0295 | 0.4349 |
| 10.0 | $\kappa_\alpha \uparrow$ | 1.2284 | -0.2733 | -0.2566 | -0.2075 | -0.4942 | -0.6956 | -1.3068 | -2.0057 |
| | $\kappa_v \uparrow$ | 0.2775 | 0.0204 | 0.0336 | 0.0444 | 0.0700 | 0.0832 | 0.0800 | 0.6090 |
| 50.0 | $\kappa_\alpha \uparrow$ | 1.2284 | -0.3635 | -0.3091 | -0.2601 | -0.5041 | -0.3879 | -1.0618 | -1.6581 |
| | $\kappa_v \uparrow$ | 0.2775 | 0.0164 | 0.0309 | 0.0410 | 0.0665 | 0.0958 | 0.0903 | 0.6183 |
| 100.0 | $\kappa_\alpha \uparrow$ | 1.2184 | -0.4001 | -0.3196 | -0.2888 | -0.3950 | -0.4705 | -1.1264 | -1.7822 |
| | $\kappa_v \uparrow$ | 0.2720 | 0.0174 | 0.0304 | 0.0394 | 0.0749 | 0.0945 | 0.0824 | 0.6108 |

## 3. Fine-Tuning Analysis

In Table 2, we display performance results for different cluster counts, separately. While the overall distribution of performance is equal for all three agreement threshold values, the average performance is maximized for the threshold value $T_{agree} = 70\%$.

Table 2: Detailed results of our Fine-Tuning Analysis, reporting scores for all cluster numbers individually.

| $D$ | $T_{agree}$ | | No Cluster | One Cluster | Two Clusters | Three Clusters | Four Clusters | Five Clusters | Six Clusters | $\Sigma$ |
|---|---|---|---|---|---|---|---|---|---|---|
| number datasets | | | 8 | 62 | 43 | 36 | 19 | 14 | 14 | 196 |
| 0.01 | 70% | $\kappa_\alpha \uparrow$ | 1.2116 | -0.1384 | -0.1254 | -0.1118 | -0.4720 | -0.3773 | -0.8346 | -0.8479 |
| | | $\kappa_v \uparrow$ | 0.2691 | 0.0261 | 0.0386 | 0.0475 | 0.0763 | 0.0964 | 0.1025 | 0.6565 |
| 0.1 | 70% | $\kappa_\alpha \uparrow$ | 1.2284 | -0.1701 | -0.0809 | -0.0881 | -0.4079 | -0.3757 | -0.6280 | -0.5223 |
| | | $\kappa_v \uparrow$ | 0.2775 | 0.0261 | 0.0426 | 0.0507 | 0.0797 | 0.1011 | 0.1105 | 0.6882 |
| 1.0 | 70% | $\kappa_\alpha \uparrow$ | 1.2284 | -0.2335 | -0.1472 | -0.0949 | -0.3544 | -0.3066 | -0.7722 | -0.6804 |
| | | $\kappa_v \uparrow$ | 0.2775 | 0.0221 | 0.0382 | 0.0488 | 0.0787 | 0.1052 | 0.1024 | 0.6729 |

## 4. Image-based Clustering

As CNN-based models proved to perform well on visual data, we include such an image-based model as a baseline to our evaluation experiments. In particular, ScatterNet [MTW*18] was proposed as an image-based similarity metric for scatter plots. However, as the model architecture of ScatterNet does not allow for image-to-image training and inference, our baseline model for image-based clustering utilizes a pre-trained U-Net [RFB15], which we further pre-train on our scatter plot images, we used for our online crowdsource study, before fine-tuning it applying identical training protocol as used for the point-based version. For fine-tuning, we use an image size of $128 \times 128$, identical to the input size of ScatterNet. Further, we pre-train the baseline using a batch size of 32, a learning rate of 1e-5, and weight decay of 0.1 using a ResNet18 [HZRS16] image encoder for 1,000 epochs applying the combined loss of contrastive loss, agreement loss, and noise loss. The loss and metric computation is done only on pixel values correlating to points. Therefore, we project the 512 points into the image domain and store the corresponding pixel coordinates, which allows us to un-project the predicted image segmentation and therefore associate class predictions to original points.

## 5. Clustering in the Wild

Both datasets PSC and SDR [SMT13] apply dimensionality reduction (DR) techniques to derive 2D data for the application of different clustering approaches. To evaluate these approaches without a potential bias of the used DR technique, we collect a third dataset without applying DR randomly sampling datasets from data.gov. The dimensionality of these datasets ranges from two to more than ten dimensions. Since we want to avoid the application of DR, we convert multidimensional data to bivariate data by randomly selecting two dimensions, as done by [MTW*18]. After visual inspection of the resulting scatterplots, we decide to crowdsource annotations from 20 human raters per stimuli, rather than only 5 resulting in 50 raters participating in the crowdsource study. We use the same web application described in the main paper collecting human clustering for 50 stimuli. Finally, we use the best model from the main paper and infer clustering and agreement predictions reporting results in Table 3 and Table 8, respectively. Looking at the results, we can see that HPSCAN's prediction slightly improves human rater agreement, indicated by a positive value of $\kappa_\alpha$. HPSCAN shows best scores for $\kappa_v$ and $\kappa_n$ amongst all competing clustering techniques, indicating well-aligned clustering prediction to human judgment. In Figure 5, we present qualitative results for HPSCAN, and ten state-of-the-art cluster techniques, evaluated on the Data.gov dataset, showing superior performance of HPSCAN in comparison to existing clustering techniques.

## 6. Data Augmentation

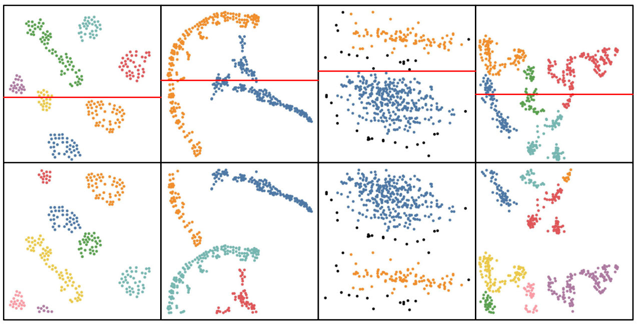

Figure 2: This depiction demonstrates our random crop data augmentation for the vertical case. In the top row, we show annotations for four stimuli and the corresponding line, where each stimulus gets cut and transformed as described below. The bottom row shows the result of our random crop data augmentation strategy used during the training of HPSCAN. Note, that in some cases the number of clusters increased, due to the cutting line going through a cluster.

Table 3: Comparison between HPSCAN and ten state-of-the-art clustering techniques using the Data.gov test dataset. Some cluster techniques do not compute outliers, for which we omit to evaluate $\kappa_n$. Results highlighted with a * are from clustering techniques, that require priors about number of clusters, which is extracted from the ground truth annotation.

| | HPSCAN | Baseline | DBSCAN [EKSX*96] | OPTICS [ABKS99] | Ward [ML11] | Mean Shift [CM02] | Affinity Propagation [FD07] | Spectral Clustering [NJW01] | Agglomerative Clustering [MW17] | BIRCH [ZRL97] | K-means [HW79] | Gaussian Mixture Model [BCRR97] |
|---|---|---|---|---|---|---|---|---|---|---|---|---|
| Evaluation on Data.gov | | | | | | | | | | | | |
| $\kappa_\alpha \uparrow$ | **1.78** | -3.60 | 1.71 | -5.20 | -3.88* | 0.45 | -6.76 | -3.88* | -0.38 | -0.88 | -3.88* | -3.88* |
| $\kappa_v \uparrow$ | **0.81** | 0.46 | 0.79 | 0.51 | 0.70* | 0.79 | 0.55 | 0.70* | 0.69 | 0.69 | 0.70* | 0.70* |
| $\kappa_n \uparrow$ | 26.74% | 13.12% | **45.42%** | 19.66% | - | - | - | - | - | - | - | - |

*The ground truth number of cluster was given to compute these scores.

In the following, we describe our random crop data augmentation strategy for point clouds, see Figure 2. This transformation can be computed in vertical or horizontal directions. We are going to describe the algorithm for the vertical direction, and for the horizontal case, all operations need to be performed along the x-axis. First, the algorithm chooses a random value $P_y$ on the y-axis. All points with smaller $y$ values than $P_y$ belong to the TOP side, and all points with equal or higher $y$ values belong o the BOTTOM side. Then all points from the TOP side are moved to the BOTTOM side and vice versa ensuring enough space in between the moved points to avoid merging clusters. Note, that points do not get mirrored, only moved from one side to the other. Next, the algorithm updates cluster IDs for all clusters that got cut during this process, so that no cluster ID repeats from one side to the other.

## 7. Investigation of Model Performance for different DR

To investigate the effect of dimension reduction in PSC, we compute performance metrics for the used DR technique separately. In Table 4, we provide results for our collected HPSCAN test dataset and the SDR [SMT13] dataset. Looking at the results, there appears to be no difference in performance for the HPSCAN test dataset. This is also the case for the SDR [SMT13] dataset. However, the results for SDR [SMT13] show some differences for RobPCA and GlimmerMDS regarding the $\kappa_\alpha$ index. While looking at the $\kappa_v$ index, these differences can not be observed. The results of this experiment suggest, that the used dimension reduction technique does not affect the performance of HPSCAN.

## 8. Detailed Quantitative Evaluation

In this section, we provide detailed quantitative evaluation results for HPSCAN and competing clustering techniques. To provide more details about cluster scores, we also compute the Silhouette cluster index [Rou87] and Calinski-Harabasz index [CH74], denoted as $\kappa_s$ and $\kappa_{ch}$. The Calinski-Harabasz Index is defined as:

$$\kappa_{ch} = \left[ \frac{\sum_{k=1}^{K} n_k ||c_k - c||^2}{K-1} \right] / \left[ \frac{\sum_{k=1}^{K} \sum_{i=1}^{n_k} ||d_i - c_k||^2}{N-K} \right] \quad (1)$$

where $K$ is the number of clusters, $n_k$ and $c_k$ are the number of points and centroid of the $k^{th}$ cluster respectively, $c$ is the global centroid, $N$ is the total number of points.

Table 4: DR-specific Performance Evaluation

| DR Technique | | No Cluster | One Clusters | Two Clusters | Three Clusters | Four Clusters | Five Clusters | Six Clusters | Ø |
|---|---|---|---|---|---|---|---|---|---|
| HPSCAN test dataset | | | | | | | | | |
| t-SNE | $\kappa_\alpha \uparrow$ | 2.9282 | -11.4216 | -0.7985 | -1.8887 | -0.6505 | -1.8059 | -3.5778 | -2.4593 |
| | $\kappa_v \uparrow$ | 0.9109 | 0.3388 | 0.6928 | 0.6750 | 0.6545 | 0.5359 | 0.6067 | 0.6307 |
| PCA | $\kappa_\alpha \uparrow$ | 4.1033 | -1.3179 | -2.1740 | 0.4484 | -9.6511 | -2.4514 | -2.9736 | -2.0023 |
| | $\kappa_v \uparrow$ | 0.8437 | 0.7355 | 0.7355 | 0.7909 | 0.3954 | 0.5723 | 0.5834 | 0.6652 |
| SDR [SMT13] dataset | | | | | | | | | |
| t-SNE | $\kappa_\alpha \uparrow$ | -0.3859 | 1.4008 | 2.1157 | -1.4417 | -4.0444 | -2.4633 | -1.7130 | -0.9331 |
| | $\kappa_v \uparrow$ | 0.8764 | 0.6761 | 0.6527 | 0.8106 | 0.5745 | 0.6483 | 0.4469 | 0.6694 |
| PCA | $\kappa_\alpha \uparrow$ | -1.9474 | 0.4879 | 0.5659 | -1.5698 | - | -6.5634 | - | -1.8054 |
| | $\kappa_v \uparrow$ | 0.8115 | 0.7216 | 0.6801 | 0.6239 | - | 0.5801 | - | 0.6834 |
| RobPCA | $\kappa_\alpha \uparrow$ | -3.0118 | -1.6462 | 0.5774 | 0.1871 | 1.0537 | - | - | -0.5680 |
| | $\kappa_v \uparrow$ | 0.9733 | 0.5456 | 0.6785 | 0.6362 | 0.4178 | - | - | 0.6503 |
| GlimmerMDS | $\kappa_\alpha \uparrow$ | -1.4394 | -1.7797 | -0.9910 | -0.8417 | - | - | - | -1.2629 |
| | $\kappa_v \uparrow$ | 0.9753 | 0.6671 | 0.5534 | 0.6432 | - | - | - | 0.7097 |

The Silhouette cluster index is defined like the following:

$$\kappa_s = \frac{b(p_i) - a(p_i)}{max(a(p_i), b(p_i))}, |C_I| > 1 \quad (2)$$

where $a$ is the mean distance between the point $p_i$ and all other data in the same cluster and $b$ relates to the smallest mean distance of $p_i$ to all points in any other cluster.

## 9. Detailed Qualitative Evaluation

In this section, we report further qualitative results for HPSCAN and existing clustering techniques on our test dataset, in Figure 3 and SDR [SMT13] dataset, which can be seen in Figure 4. We provide cluster results for five and eight stimuli, respectively, along with a human annotation, that got the highest agreement score, computed among 5 human judgments. We can show, that HPSCAN provides cluster predictions, which align well with human-perceived clustering results.

In a second experiment, we collected annotations for stimuli, that originate from bi-variate data with the absence of dimension reduction. This experiment further investigates the generalization capacity of HPSCAN to data out of distribution. In Figure 5, we provide visual results for eight stimuli, originating from the Data.gov

Table 5: Detailed quantitative evaluation results of multiple clustering techniques for PSC dataset. We weight individual cluster scores by the number of samples to counteract differences in cluster numbers. The last column computes the weighted sum.

| Method | | No Cluster | One Cluster | Two Cluster | Three Cluster | Four Cluster | Five Cluster | Six Cluster | Σ |
|---|---|---|---|---|---|---|---|---|---|
| Human | $\kappa_s$ | 0.0787 | 0.0229 | 0.0321 | 0.0331 | 0.0561 | 0.0713 | 0.0792 | 0.3734 |
| | $\kappa_{ch}$ | 19129.1158 | 0.0127 | 180.3861 | 0.0417 | 0.0677 | 0.1168 | 0.1158 | 19309.8565 |
| HPSCAN | $\kappa_\alpha$ | 1.2284 | -0.1701 | -0.0805 | -0.0888 | -0.4099 | -0.3752 | -0.6274 | -0.5236 |
| | $\kappa_v$ | 0.2775 | 0.0261 | 0.0426 | 0.0507 | 0.0796 | 0.1011 | 0.1106 | 0.6881 |
| | $\kappa_n$ | 26.17% | 2.67% | 3.81% | 4.23% | 7.61% | 7.79% | 7.39% | 59.68% |
| | $\kappa_s$ | - | 0.0215 | 0.0278 | 0.0322 | 0.0528 | 0.0654 | 0.0694 | 0.2690 |
| | $\kappa_{ch}$ | - | 0.0136 | 0.0343 | 0.0346 | 0.0533 | 0.0849 | 0.0616 | 0.2823 |
| Baseline | $\kappa_\alpha$ | 1.2046 | -0.2663 | -0.3437 | -0.3025 | -0.5942 | -0.8389 | -1.2611 | -2.4023 |
| | $\kappa_v$ | 0.2133 | 0.0188 | 0.0276 | 0.0365 | 0.0622 | 0.0744 | 0.0731 | 0.5058 |
| | $\kappa_n$ | 26.13% | 1.30% | 1.80% | 1.73% | 1.26% | 1.38% | 2.53% | 36.13% |
| | $\kappa_s$ | 0.0422 | 0.0164 | 0.0211 | 0.0240 | 0.0267 | 0.0433 | 0.0281 | 0.2019 |
| | $\kappa_{ch}$ | 0.0018 | 0.0097 | 0.0210 | 0.0302 | 0.0349 | 0.0503 | 0.0333 | 0.1811 |
| Affinity Propagation | $\kappa_\alpha$ | -6.5945 | -0.6784 | -0.7489 | -0.5841 | -0.8804 | -0.4861 | -0.3937 | -10.3662 |
| | $\kappa_v$ | 0.1128 | 0.0125 | 0.0126 | 0.0205 | 0.0436 | 0.0967 | 0.0919 | 0.3906 |
| | $\kappa_n$ | 6.08% | 3.74% | 5.33% | 6.64% | 12.58% | 16.69% | 17.12% | 68.17% |
| | $\kappa_s$ | 0.2052 | 0.0231 | 0.0359 | 0.0424 | 0.0766 | 0.1112 | 0.1097 | 0.6040 |
| | $\kappa_{ch}$ | 1.3315 | 11.7357 | 401.6969 | 0.2280 | 0.2638 | 0.4465 | 0.4436 | 416.1459 |
| Agglomerative Clustering | $\kappa_\alpha$ | -2.0557 | -0.1311 | -0.0634 | -0.2337 | -1.0482 | -1.8123 | -1.6797 | -7.0241 |
| | $\kappa_v$ | 0.1369 | 0.0170 | 0.0394 | 0.0360 | 0.0478 | 0.0378 | 0.0688 | 0.3837 |
| | $\kappa_n$ | 6.08% | 3.74% | 5.33% | 6.64% | 12.58% | 16.69% | 17.12% | 68.17% |
| | $\kappa_s$ | 0.1290 | 0.0282 | 0.0350 | 0.0395 | 0.0643 | 0.0840 | 0.0865 | 0.4665 |
| | $\kappa_{ch}$ | 0.0996 | 0.0154 | 0.0412 | 0.0370 | 0.0466 | 0.0493 | 0.0637 | 0.3530 |
| Birch | $\kappa_\alpha$ | -2.7225 | -0.1538 | -0.1013 | -0.3114 | -1.0233 | -1.5820 | -1.7853 | -7.6797 |
| | $\kappa_v$ | 0.1230 | 0.0223 | 0.0386 | 0.0356 | 0.0527 | 0.0515 | 0.0529 | 0.3765 |
| | $\kappa_n$ | 6.08% | 3.74% | 5.33% | 6.64% | 12.58% | 16.69% | 17.12% | 68.17% |
| | $\kappa_s$ | 0.1379 | 0.0244 | 0.0338 | 0.0346 | 0.0601 | 0.0859 | 0.0831 | 0.4598 |
| | $\kappa_{ch}$ | 0.1205 | 0.0128 | 0.0582 | 0.0332 | 0.0561 | 0.0641 | 0.0658 | 0.4106 |
| DBSCAN | $\kappa_\alpha$ | -3.1053 | 0.0272 | 0.0562 | -0.0939 | -0.2128 | -0.1228 | -0.6775 | -4.1290 |
| | $\kappa_v$ | 0.1357 | 0.0331 | 0.0509 | 0.0528 | 0.0920 | 0.1244 | 0.1302 | 0.6190 |
| | $\kappa_n$ | 2.00% | 2.71% | 4.24% | 5.46% | 10.44% | 14.56% | 12.71% | 52.12% |
| | $\kappa_s$ | 0.1923 | 0.0279 | 0.0355 | 0.0372 | 0.0644 | 0.0782 | 0.0796 | 0.5151 |
| | $\kappa_{ch}$ | 16398.8919 | 0.0115 | 204.1579 | 0.0283 | 0.0837 | 0.1100 | 0.0981 | 16603.3815 |
| Gaussian Mixture Model | $\kappa_\alpha$ | 1.2284 | 0.0182 | -0.4416 | -0.7487 | -1.9552 | -2.9131 | -4.0051 | -8.8171 |
| | $\kappa_v$ | 0.2775 | 0.0365 | 0.0381 | 0.0391 | 0.0573 | 0.0660 | 0.0540 | 0.5685 |
| | $\kappa_n$ | 6.08% | 3.74% | 5.33% | 6.64% | 12.58% | 16.69% | 17.12% | 68.17% |
| | $\kappa_s$ | - | - | - | - | - | - | - | - |
| | $\kappa_{ch}$ | - | - | - | - | - | - | - | - |
| K-Means | $\kappa_\alpha$ | 1.2284 | 0.0182 | -0.4416 | -0.7487 | -1.9552 | -2.9131 | -4.0051 | -8.8171 |
| | $\kappa_v$ | 0.2775 | 0.0365 | 0.0381 | 0.0391 | 0.0573 | 0.0660 | 0.0540 | 0.5685 |
| | $\kappa_n$ | 6.08% | 3.74% | 5.33% | 6.64% | 12.58% | 16.69% | 17.12% | 68.17% |
| | $\kappa_s$ | - | - | - | - | - | - | - | - |
| | $\kappa_{ch}$ | - | - | - | - | - | - | - | - |
| Mean Shift | $\kappa_\alpha$ | -5.2427 | -0.3799 | -0.3122 | -0.1716 | -0.4680 | -0.1428 | -0.1817 | -6.8989 |
| | $\kappa_v$ | 0.1193 | 0.0195 | 0.0313 | 0.0446 | 0.0690 | 0.1141 | 0.1294 | 0.5272 |
| | $\kappa_n$ | 6.08% | 3.74% | 5.33% | 6.64% | 12.58% | 16.69% | 17.12% | 68.17% |
| | $\kappa_s$ | 0.1780 | 0.0280 | 0.0397 | 0.0434 | 0.0754 | 0.1076 | 0.1072 | 0.5794 |
| | $\kappa_{ch}$ | 14346.9991 | 0.0609 | 180.4853 | 0.0824 | 0.1383 | 0.1945 | 0.1972 | 14528.1578 |
| OPTICS | $\kappa_\alpha$ | -2.3323 | -0.5114 | -0.4835 | -0.4264 | -0.5451 | -0.0325 | -1.2277 | -5.5591 |
| | $\kappa_v$ | 0.2272 | 0.0103 | 0.0204 | 0.0303 | 0.0595 | 0.1238 | 0.0898 | 0.5612 |
| | $\kappa_n$ | 8.95% | 0.97% | 0.66% | 0.81% | 1.79% | 3.47% | 4.65% | 21.29% |
| | $\kappa_s$ | 0.1373 | 0.0095 | 0.0203 | 0.0267 | 0.0442 | 0.0796 | 0.0725 | 0.3900 |
| | $\kappa_{ch}$ | 0.4921 | 0.0108 | 0.0466 | 0.0423 | 0.0426 | 0.1010 | 0.0835 | 0.8189 |
| Spectral Clustering | $\kappa_\alpha$ | 1.2284 | 0.0182 | -0.4416 | -0.7487 | -1.9552 | -2.9131 | -4.0051 | -8.8171 |
| | $\kappa_v$ | 0.2775 | 0.0365 | 0.0381 | 0.0391 | 0.0573 | 0.0660 | 0.0540 | 0.5685 |
| | $\kappa_n$ | 6.08% | 3.74% | 5.33% | 6.64% | 12.58% | 16.69% | 17.12% | 68.17% |
| | $\kappa_s$ | - | - | - | - | - | - | - | - |
| | $\kappa_{ch}$ | - | - | - | - | - | - | - | - |
| Ward | $\kappa_\alpha$ | 1.2284 | 0.0182 | -0.4416 | -0.7487 | -1.9552 | -2.9131 | -4.0051 | -8.8171 |
| | $\kappa_v$ | 0.2775 | 0.0365 | 0.0381 | 0.0391 | 0.0573 | 0.0660 | 0.0540 | 0.5685 |
| | $\kappa_n$ | 6.08% | 3.74% | 5.33% | 6.64% | 12.58% | 16.69% | 17.12% | 68.17% |
| | $\kappa_s$ | - | - | - | - | - | - | - | - |
| | $\kappa_{ch}$ | - | - | - | - | - | - | - | - |

Table 6: Detailed quantitative evaluation results of multiple clustering techniques for the SDR [SMT13] test dataset. We weight individual cluster scores by the number of samples to counteract differences in cluster numbers. The last column computes the weighted sum.

| Method | | No Cluster | One Cluster | Two Cluster | Three Cluster | Σ |
|---|---|---|---|---|---|---|
| Human | $\kappa_s$ | 0.0437 | 0.0494 | 0.0701 | 0.1617 | 0.3249 |
| | $\kappa_{ch}$ | 0.0257 | 1.0302 | 0.0621 | 0.2542 | 1.3722 |
| HPSCAN | $\kappa_\alpha$ | -0.2831 | -0.1778 | -0.0552 | -0.8269 | -1.3431 |
| | $\kappa_v$ | 0.1675 | 0.0762 | 0.1291 | 0.2671 | 0.6398 |
| | $\kappa_n$ | 15.00% | 6.20% | 9.39% | 15.69% | 46.28% |
| | $\kappa_s$ | -0.0022 | 0.0280 | 0.0483 | 0.1157 | 0.1899 |
| | $\kappa_{ch}$ | 0.0063 | 1.1077 | 0.0343 | 0.1312 | 1.2796 |
| Baseline | $\kappa_\alpha$ | 0.2088 | -0.1843 | -1.2141 | -4.1567 | -5.3463 |
| | $\kappa_v$ | 0.1751 | 0.0709 | 0.0810 | 0.1073 | 0.4342 |
| | $\kappa_n$ | 15.68% | 4.88% | 5.49% | 7.82% | 33.86% |
| | $\kappa_s$ | -0.0263 | 0.0254 | 0.0258 | 0.0324 | 0.0572 |
| | $\kappa_{ch}$ | 0.0023 | 0.1100 | 0.0132 | 0.0394 | 0.1648 |
| Affinity Propagation | $\kappa_\alpha$ | -5.6719 | -2.2500 | -1.6211 | -3.4982 | -13.0413 |
| | $\kappa_v$ | 0.1189 | 0.0258 | 0.0494 | 0.1192 | 0.3133 |
| | $\kappa_n$ | 2.73% | 9.56% | 16.72% | 38.05% | 67.07% |
| | $\kappa_s$ | 0.0762 | 0.0616 | 0.0967 | 0.1897 | 0.4243 |
| | $\kappa_{ch}$ | 0.0984 | 1.0757 | 0.1891 | 0.4810 | 1.8441 |
| Agglomerative Clustering | $\kappa_\alpha$ | -2.2514 | -0.4061 | -0.5355 | -2.6537 | -5.8467 |
| | $\kappa_v$ | 0.1228 | 0.0445 | 0.0903 | 0.1678 | 0.4255 |
| | $\kappa_n$ | 2.73% | 9.56% | 16.72% | 38.05% | 67.07% |
| | $\kappa_s$ | 0.0646 | 0.0737 | 0.1093 | 0.2256 | 0.4732 |
| | $\kappa_{ch}$ | 0.0503 | 1.0215 | 0.0772 | 0.1380 | 1.2870 |
| Birch | $\kappa_\alpha$ | -2.5801 | -0.3985 | -0.5621 | -2.9256 | -6.4663 |
| | $\kappa_v$ | 0.1221 | 0.0595 | 0.0948 | 0.1825 | 0.4589 |
| | $\kappa_n$ | 2.73% | 9.56% | 16.72% | 38.05% | 67.07% |
| | $\kappa_s$ | 0.0639 | 0.0580 | 0.0976 | 0.1895 | 0.4091 |
| | $\kappa_{ch}$ | 0.0539 | 0.0389 | 0.0788 | 0.1547 | 0.3263 |
| DBSCAN | $\kappa_\alpha$ | -0.7725 | 0.0751 | -0.5057 | -1.9888 | -3.1919 |
| | $\kappa_v$ | 0.1277 | 0.0662 | 0.0992 | 0.2052 | 0.4983 |
| | $\kappa_n$ | 1.49% | 3.51% | 5.67% | 17.69% | 28.36% |
| | $\kappa_s$ | 0.0357 | 0.0588 | 0.0884 | 0.2154 | 0.3984 |
| | $\kappa_{ch}$ | 0.1351 | 1.1040 | 0.0394 | 0.2088 | 1.4873 |
| Gaussian Mixture Model | $\kappa_\alpha$ | 0.2679 | 0.1537 | -1.3338 | -6.2959 | -7.2080 |
| | $\kappa_v$ | 0.1768 | 0.1140 | 0.1279 | 0.1988 | 0.6175 |
| | $\kappa_n$ | 2.73% | 9.56% | 16.72% | 38.05% | 67.07% |
| | $\kappa_s$ | - | - | - | - | 0.0000 |
| | $\kappa_{ch}$ | - | - | - | - | 0.0000 |
| K-Means | $\kappa_\alpha$ | 0.2679 | 0.1537 | -1.3338 | -6.2959 | -7.2080 |
| | $\kappa_v$ | 0.1768 | 0.1140 | 0.1279 | 0.1988 | 0.6175 |
| | $\kappa_n$ | 2.73% | 9.56% | 16.72% | 38.05% | 67.07% |
| | $\kappa_s$ | - | - | - | - | 0.0000 |
| | $\kappa_{ch}$ | - | - | - | - | 0.0000 |
| Mean Shift | $\kappa_\alpha$ | -3.8251 | -0.8311 | -0.3315 | -0.2907 | -5.2785 |
| | $\kappa_v$ | 0.1256 | 0.0559 | 0.1195 | 0.2956 | 0.5965 |
| | $\kappa_n$ | 2.73% | 9.56% | 16.72% | 38.05% | 67.07% |
| | $\kappa_s$ | 0.0700 | 0.0725 | 0.1174 | 0.2470 | 0.5069 |
| | $\kappa_{ch}$ | 0.0782 | 1.1913 | 0.1347 | 0.3424 | 1.7466 |
| OPTICS | $\kappa_\alpha$ | -0.7859 | -0.4013 | -0.7339 | -1.2278 | -3.1490 |
| | $\kappa_v$ | 0.1531 | 0.0758 | 0.1072 | 0.2603 | 0.5964 |
| | $\kappa_n$ | 6.22% | 6.71% | 7.95% | 15.22% | 36.11% |
| | $\kappa_s$ | 0.0198 | 0.0245 | 0.0581 | 0.1690 | 0.2714 |
| | $\kappa_{ch}$ | 0.0186 | 0.0261 | 0.0572 | 0.2470 | 0.3489 |
| Spectral Clustering | $\kappa_\alpha$ | 0.2679 | 0.1537 | -1.3338 | -6.2959 | -7.2080 |
| | $\kappa_v$ | 0.1768 | 0.1140 | 0.1279 | 0.1988 | 0.6175 |
| | $\kappa_n$ | 2.73% | 9.56% | 16.72% | 38.05% | 67.07% |
| | $\kappa_s$ | - | - | - | - | 0.0000 |
| | $\kappa_{ch}$ | - | - | - | - | 0.0000 |
| Ward | $\kappa_\alpha$ | 0.2679 | 0.1537 | -1.3338 | -6.2959 | -7.2080 |
| | $\kappa_v$ | 0.1768 | 0.1140 | 0.1279 | 0.1988 | 0.6175 |
| | $\kappa_n$ | 2.73% | 9.56% | 16.72% | 38.05% | 67.07% |
| | $\kappa_s$ | - | - | - | - | 0.0000 |
| | $\kappa_{ch}$ | - | - | - | - | 0.0000 |

Table 7: Detailed quantitative evaluation results of multiple clustering techniques for the Data.gov test dataset. We weight individual cluster scores by the number of samples to counteract differences in cluster numbers. The last column computes the weighted sum.

| Method | | No Cluster | One Cluster | Two Cluster | Three Cluster | Σ |
|---|---|---|---|---|---|---|
| Human | $\kappa_s$ | 0.3166 | 0.0927 | 0.1150 | 0.2190 | 0.7432 |
| | $\kappa_{ch}$ | 2473.8743 | 0.0972 | 0.7617 | 1.7457 | 2476.4789 |
| HPSCAN | $\kappa_\alpha$ | -0.0836 | -0.0491 | -0.1294 | 2.0439 | 1.7817 |
| | $\kappa_v$ | 0.2217 | 0.0794 | 0.1126 | 0.3967 | 0.8103 |
| | $\kappa_n$ | 10.48% | 3.92% | 3.28% | 9.06% | 26.74% |
| | $\kappa_s$ | 0.1581 | 0.0667 | 0.0837 | 0.2546 | 0.5632 |
| | $\kappa_{ch}$ | 0.9600 | 0.0332 | 0.2802 | 0.9467 | 2.2201 |
| Baseline | $\kappa_\alpha$ | -0.8471 | -0.2879 | -0.5536 | -1.9067 | -3.5953 |
| | $\kappa_v$ | 0.2151 | 0.0360 | 0.0737 | 0.1361 | 0.4609 |
| | $\kappa_n$ | 8.90% | 0.50% | 1.67% | 2.05% | 13.12% |
| | $\kappa_s$ | 0.1737 | 0.0450 | 0.0566 | 0.0642 | 0.3395 |
| | $\kappa_{ch}$ | 0.1732 | 0.0163 | 0.1608 | 0.0377 | 0.3881 |
| Affinity Propagation | $\kappa_\alpha$ | -3.4589 | -1.8719 | -0.8792 | -0.5513 | -6.7613 |
| | $\kappa_v$ | 0.2143 | 0.0274 | 0.0840 | 0.2314 | 0.5571 |
| | $\kappa_n$ | 21.25% | 11.05% | 14.79% | 38.89% | 85.98% |
| | $\kappa_s$ | 0.1734 | 0.0670 | 0.1166 | 0.2473 | 0.6043 |
| | $\kappa_{ch}$ | 4315.9548 | 37.9748 | 1.7601 | 4.4389 | 4360.1287 |
| Agglomerative Clustering | $\kappa_\alpha$ | -0.5202 | 0.0339 | -0.2044 | 0.3104 | -0.3803 |
| | $\kappa_v$ | 0.2743 | 0.0701 | 0.0890 | 0.2527 | 0.6862 |
| | $\kappa_n$ | 21.25% | 11.05% | 14.79% | 38.89% | 85.98% |
| | $\kappa_s$ | 0.2527 | 0.0929 | 0.1239 | 0.2596 | 0.7291 |
| | $\kappa_{ch}$ | 1190.8505 | 0.0969 | 0.7751 | 0.3258 | 1192.0483 |
| Birch | $\kappa_\alpha$ | -0.5168 | -0.0078 | -0.5697 | 0.2177 | -0.8766 |
| | $\kappa_v$ | 0.2741 | 0.0855 | 0.0885 | 0.2462 | 0.6944 |
| | $\kappa_n$ | 21.25% | 11.05% | 14.79% | 38.89% | 85.98% |
| | $\kappa_s$ | 0.2422 | 0.0813 | 0.1249 | 0.2555 | 0.7039 |
| | $\kappa_{ch}$ | 1575.6255 | 0.1293 | 0.8723 | 0.3285 | 1576.9556 |
| DBSCAN | $\kappa_\alpha$ | -0.0158 | 0.0150 | 0.1980 | 1.5123 | 1.7095 |
| | $\kappa_v$ | 0.2352 | 0.0898 | 0.1288 | 0.3396 | 0.7934 |
| | $\kappa_n$ | 8.42% | 3.76% | 5.82% | 27.41% | 45.42% |
| | $\kappa_s$ | 0.2541 | 0.0841 | 0.1254 | 0.3260 | 0.7896 |
| | $\kappa_{ch}$ | 2165.5466 | 0.0980 | 1.0733 | 7.8160 | 2174.5340 |
| Gaussian Mixture Model | $\kappa_\alpha$ | -0.0666 | -0.2214 | -0.5994 | -2.9916 | -3.8790 |
| | $\kappa_v$ | 0.2651 | 0.0998 | 0.1190 | 0.2166 | 0.7005 |
| | $\kappa_n$ | 21.25% | 11.05% | 14.79% | 38.89% | 85.98% |
| | $\kappa_s$ | - | - | - | - | 0.0000 |
| | $\kappa_{ch}$ | - | - | - | - | 0.0000 |
| K-Means | $\kappa_\alpha$ | -0.0666 | -0.2214 | -0.5994 | -2.9916 | -3.8790 |
| | $\kappa_v$ | 0.2651 | 0.0998 | 0.1190 | 0.2166 | 0.7005 |
| | $\kappa_n$ | 21.25% | 11.05% | 14.79% | 38.89% | 85.98% |
| | $\kappa_s$ | - | - | - | - | 0.0000 |
| | $\kappa_{ch}$ | - | - | - | - | 0.0000 |
| Mean Shift | $\kappa_\alpha$ | -0.8072 | -0.1715 | -0.4568 | 1.8844 | 0.4490 |
| | $\kappa_v$ | 0.2347 | 0.0790 | 0.0998 | 0.3781 | 0.7915 |
| | $\kappa_n$ | 21.25% | 11.05% | 14.79% | 38.89% | 85.98% |
| | $\kappa_s$ | 0.2617 | 0.0923 | 0.1300 | 0.3198 | 0.8038 |
| | $\kappa_{ch}$ | 2167.6133 | 0.1906 | 1.2796 | 1.9507 | 2171.0343 |
| OPTICS | $\kappa_\alpha$ | -3.4739 | -0.6318 | -1.3691 | 0.2708 | -5.2039 |
| | $\kappa_v$ | 0.0996 | 0.0656 | 0.0646 | 0.2811 | 0.5109 |
| | $\kappa_n$ | 3.30% | 4.75% | 2.97% | 8.64% | 19.66% |
| | $\kappa_s$ | 0.0951 | 0.0313 | 0.0604 | 0.2023 | 0.3891 |
| | $\kappa_{ch}$ | 756.1636 | 0.0778 | 0.5143 | 0.9925 | 757.7482 |
| Spectral Clustering | $\kappa_\alpha$ | -0.0666 | -0.2214 | -0.5994 | -2.9916 | -3.8790 |
| | $\kappa_v$ | 0.2651 | 0.0998 | 0.1190 | 0.2166 | 0.7005 |
| | $\kappa_n$ | 21.25% | 11.05% | 14.79% | 38.89% | 85.98% |
| | $\kappa_s$ | - | - | - | - | 0.0000 |
| | $\kappa_{ch}$ | - | - | - | - | 0.0000 |
| Ward | $\kappa_\alpha$ | -0.0666 | -0.2214 | -0.5994 | -2.9916 | -3.8790 |
| | $\kappa_v$ | 0.2651 | 0.0998 | 0.1190 | 0.2166 | 0.7005 |
| | $\kappa_n$ | 21.25% | 11.05% | 14.79% | 38.89% | 85.98% |
| | $\kappa_s$ | - | - | - | - | 0.0000 |
| | $\kappa_{ch}$ | - | - | - | - | 0.0000 |

dataset. In this experiment, we can show superior results of HPSCAN, that align well with human judgments, underlining the ability of HPSCAN to generalize to unseen data.

## 10. Dataset statistics

Figure Figure 6 visualizes the data point distribution separated by cluster counts. It indicates that human raters perceived three clusters or fewer while agreeing by a rate close to 80%. For evaluation, we only use data points, that got annotated with three or fewer clusters, indicated by orange bars in Figure Figure 6, as the samples contribute more than 5% to the dataset.

In Figure 7 the annotation and corresponding human rater agreement is displayed. Looking at the collected annotations, human raters mainly perceived three clusters or fewer. However, it is interesting to see, that human raters agree more for the cases when three or more clusters were selected. This directly correlates with the number of stimuli. In the case of four, five, and six clusters, only a single stimulus was ranked as such. For evaluation, we excluded those data points, since these cases contribute lower than 5% to the test dataset.

## 11. CLAMS - Human Agreement Estimation

In this experiment, we investigate human agreement for the CLAMS [JQL*24] dataset, which they collected from 18 human raters for 60 scatterplots, where each participant worked on all stimuli. The task is to separate clusters by utilizing a lasso tool which determines the clusters in the given scatterplot using the mouse. We report the dataset statistics for CLAMS in Figure 9 showing a mean agreement of 81% between human raters, indicating similar agreement rates compared to HPSCAN, SDR [SMT13] and Data.gov. Having analyzed human agreement within the CLAMS dataset, we investigate agreement estimation using HPSCAN, and therefore, we apply our best model from the fine-tune experiment in the main paper and report results in Table 8. of the main paper. The results indicate slightly better performance for CLAMS compared to the PSC, Data.gov, and SDR [SMT13] dataset, which is due to a relatively high agreement rate within the dataset.

## 12. Filter Agreement vs. Dataset size Experiment

In this experiment, we investigate the impact of increasing human agreement during training for our model performance. To do so, we use a threshold $T_{\text{agree}}$ to filter our training dataset. We start by $T_{\text{agree}} = 10\%$ and increase it in 10% steps until we reach $T_{\text{agree}} = 100\%$. For each threshold, we discard training samples, where the agreement score $\alpha(G) < T_{\text{agree}}$. In such a way, we construct 5 subsets using threshold values: $50\%, 60\%, 70\%, 80\%, 90\%$. In Figure 10, we report the number of remaining training data for each threshold, as well as the resulting average agreement score. Looking at the different dataset sizes, we chose the aforementioned 5 threshold values, to use in this experiment. We do not train a model using threshold 100%, since too few training samples would remain to expect a robust model. For threshold values below 50%, no training sample gets discarded, and we call this dataset UNFILTERED. In this experiment, we use a fixed negative momentum

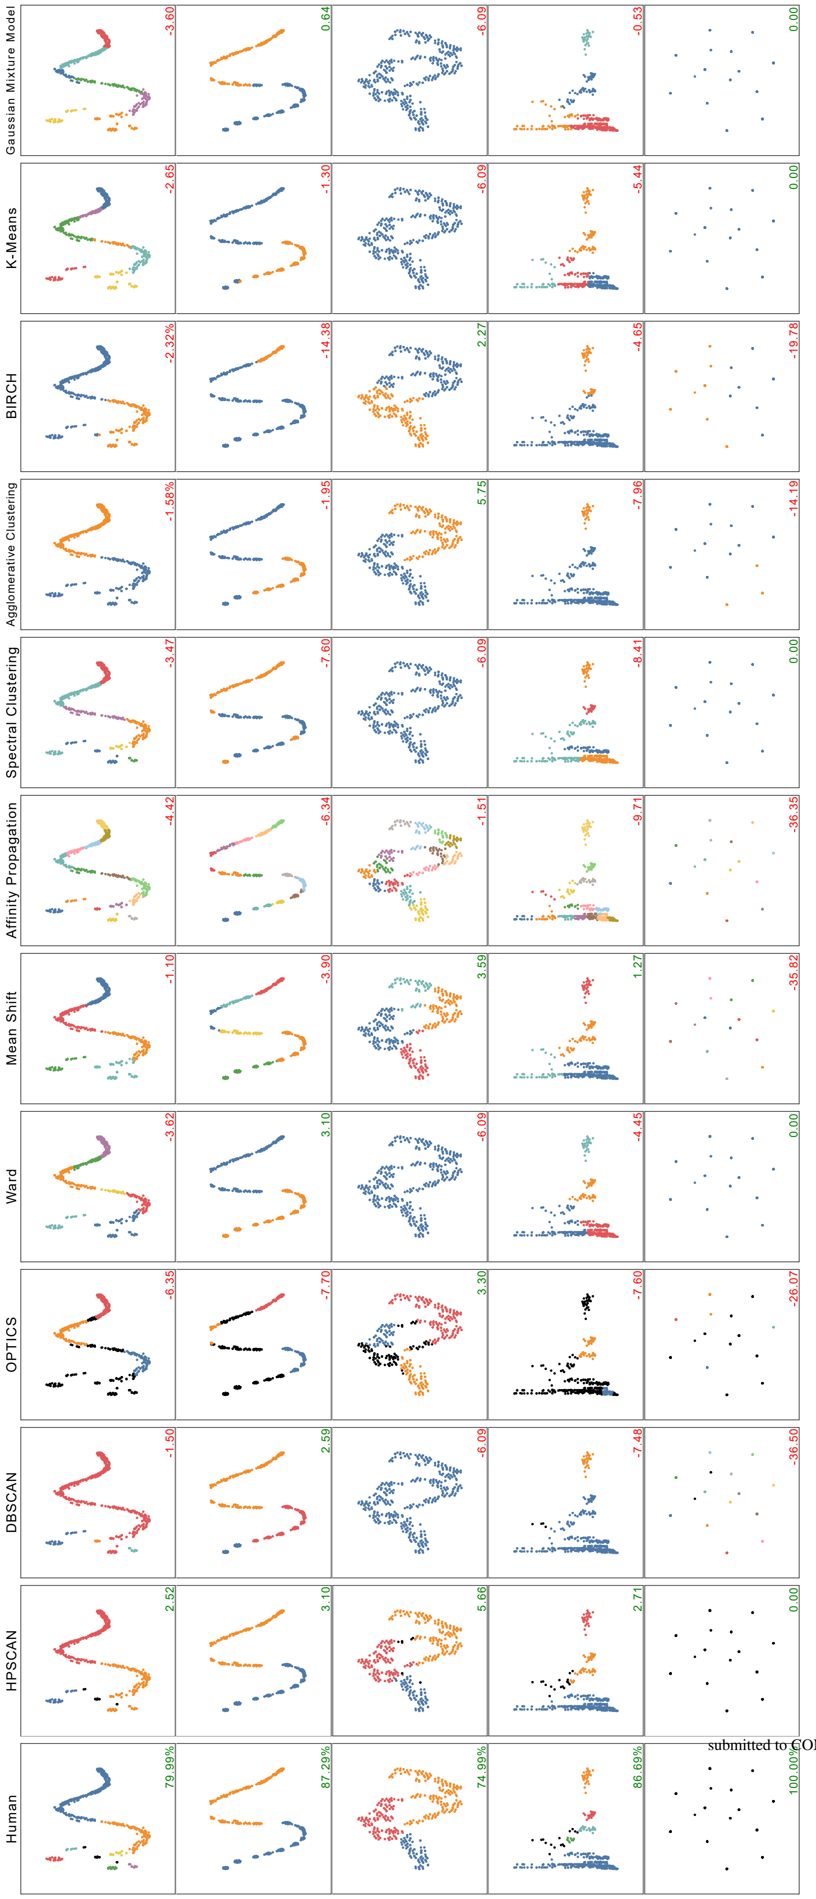




Figure 3: HPSCAN clusters scatterplots in accordance with human cluster perception.

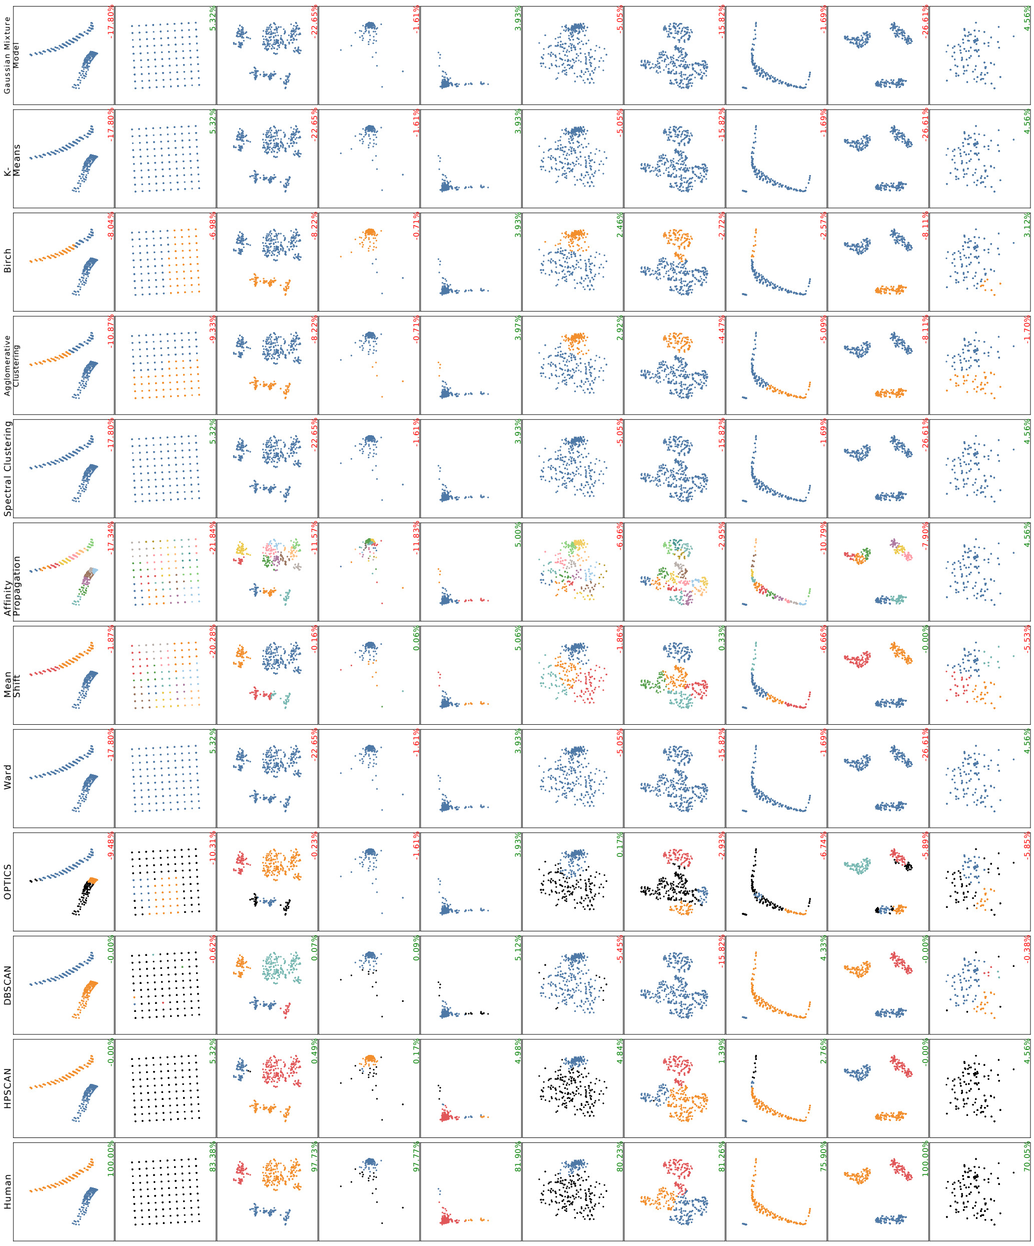


Figure 4: Qualitative evaluation results for the SDR [SMT13] dataset. Each column shows the results for a clustering technique. We compare our approach HPSCAN and ten existing clustering techniques, as well as the human rating with the maximum agreement inside the group of raters, in the first column. For each technique, the corresponding $\kappa_\alpha$ score is show in green, when the clustering improves group agreement and red, otherwise.

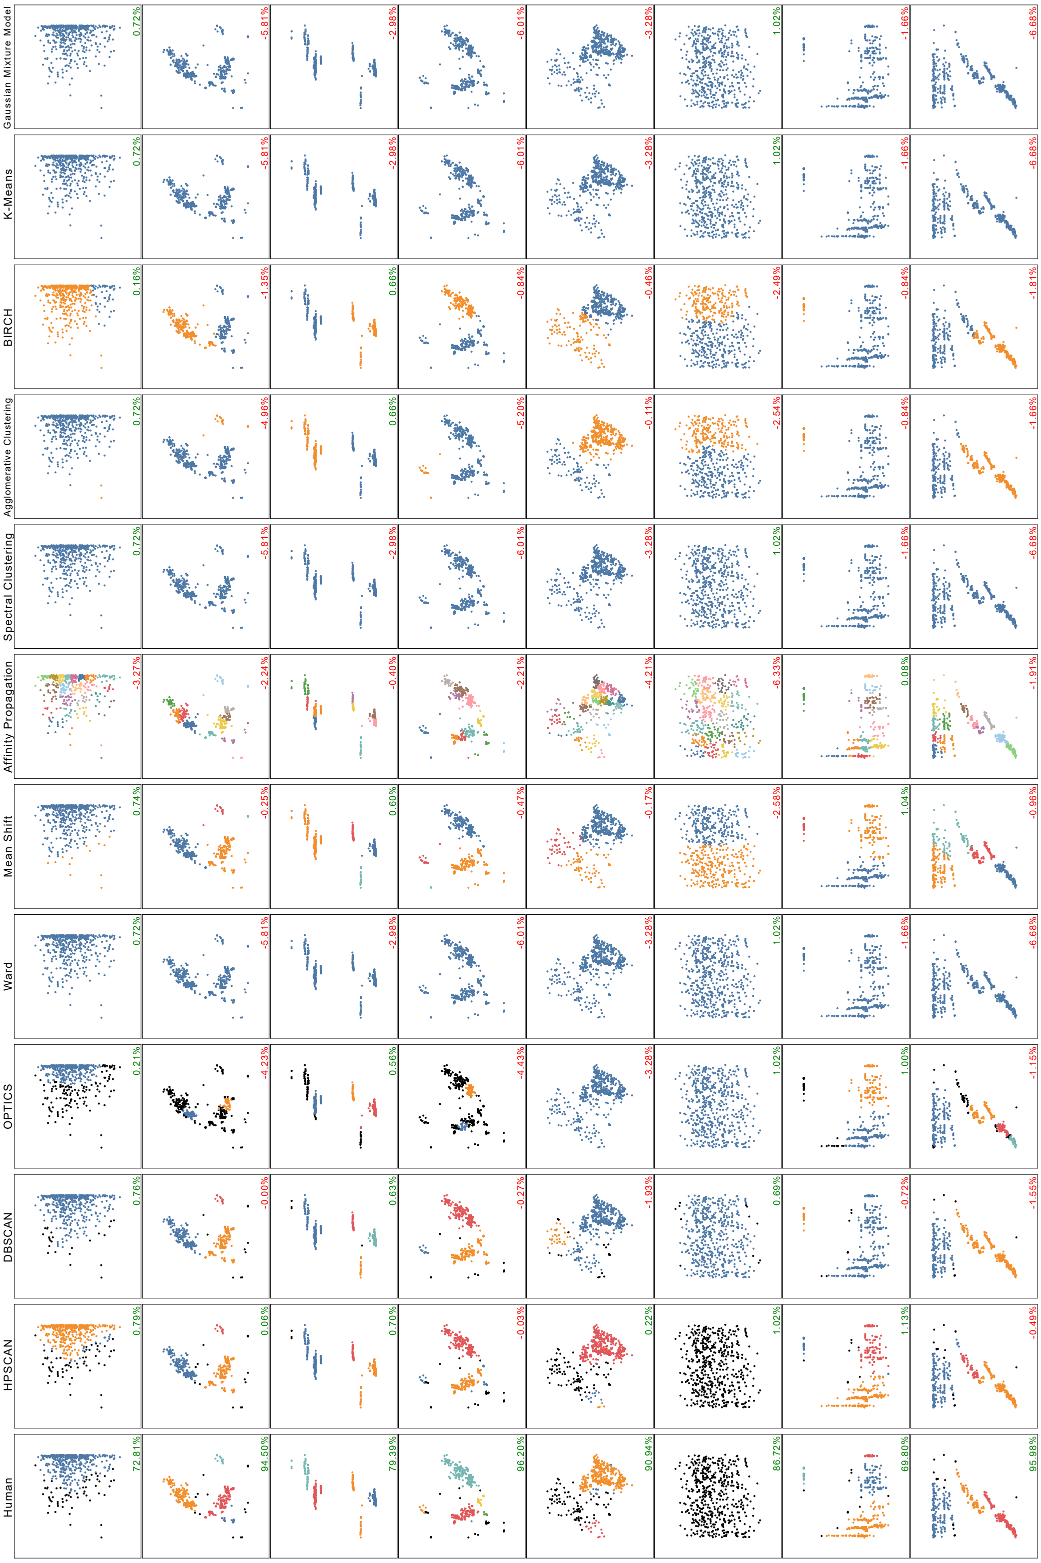


Figure 5: Qualitative evaluation results for the Data.gov dataset. Each column shows the results for a clustering technique. We compare our approach HPSCAN and ten existing clustering techniques, as well as the human rating with the maximum agreement inside the group of raters, in the first column. For each technique, the corresponding $\kappa_\alpha$ score is show in green, when the clustering improves group agreement and red, otherwise.

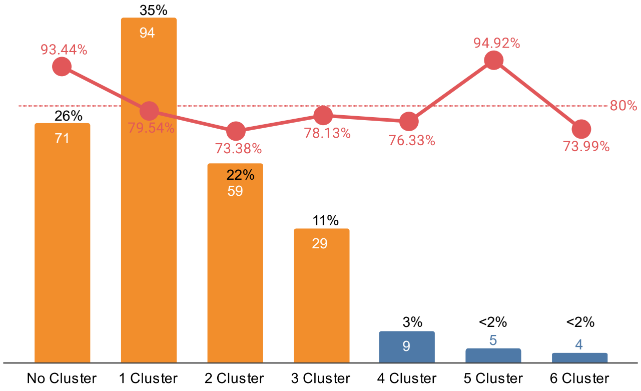


Figure 6: SDR [SMT13] consists of 272 stimuli, we show the distribution of stimuli that got annotated with a certain number of clusters. The user agreement is visualized in red for the number of clusters.

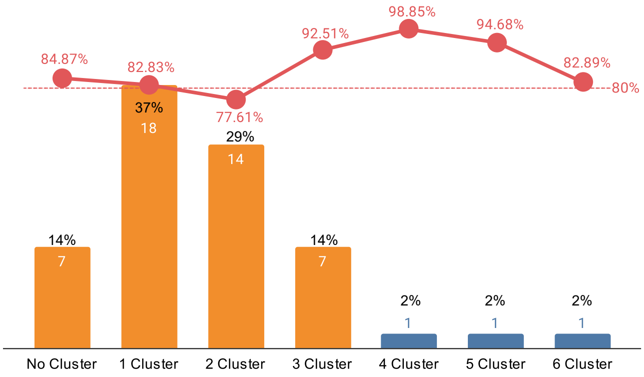


Figure 7: Data.gov consists of 50 stimuli, we show the distribution of stimuli that got annotated with a certain number of clusters. The user agreement is visualized in red for the number of clusters, respectively. Note, that for Data.gov per stimulus, 20 human raters provided clustering annotations.

$D = 50.0$ and otherwise identical hyperparameters as described in the main paper.

Further, we compare the different versions of HPSCAN trained on annotations with the high human agreement, see the middle part of Table 8. For each annotation, we computed the agreement rate and kept only annotations with an agreement score higher than a certain threshold $T$. Similarly, we compared using the best $N$ annotations, see in the bottom part of Table 8. We can show, that keeping annotations with high agreement does not increase performance results, on the contrary, it leads to worse performance compared to utilizing all available annotations.

In a second experiment, we investigate the effect of available training data after filtering for agreement between human annotators, we conduct the following experiment. We select seven threshold parameters $T = 0\%, 50\%, 60\%, 70\%, 80\%, 90\%, 100\%$ and filter our training dataset, resulting in a dataset with varying sizes:

| Test dataset | MSE | MAE |
|---|---|---|
| HPSCAN | 0.0305 | 0.1393 |
| SDR [SMT13] | 0.0317 | 0.1564 |
| CLAMS [JQL*24] | 0.0227 | 0.1286 |
| Data.gov | 0.0261 | 0.1451 |
| HPSCAN @1.0 | 0.0578 | 0.1813 |
| HPSCAN @0.9 | 0.0515 | 0.1741 |
| HPSCAN @0.8 | 0.0484 | 0.1705 |
| HPSCAN @0.7 | 0.0425 | 0.1632 |
| HPSCAN @Top-4 Agreement | 0.0497 | 0.1724 |
| HPSCAN @Top-3 Agreement | 0.0562 | 0.1784 |
| HPSCAN @Top-2 Agreement | 0.0570 | 0.1804 |

Table 8: We evaluate our model, which is trained on our dataset, for the human agreement estimation task. Top: We compute two regression metrics to measure its performance on four datasets: HPSCAN SDR [SMT13], CLAMS, and Data.gov, which consists of real and synthetic scatterplots. Middle: Four versions of HPSCAN which are trained on annotations, where only annotations with agreement score higher than $T$ are used (@T). Bottom: HPSCAN is trained with best N annotations which maximize agreement inside the group (Top-N).

| | 1171 | 1148 | 1049 | 883 | 672 | 448 | 74 |
|---|---|---|---|---|---|---|---|
| 0% | -3.18 | -3.48 | -2.93 | -3.79 | -4.61 | -5.77 | -9.54 |
| 50% | - | -3.38 | -3.48 | -3.52 | -4.61 | -5.36 | -9.35 |
| 60% | - | - | -2.96 | -3.75 | -4.59 | -5.43 | -9.98 |
| 70% | - | - | - | -3.63 | -5.06 | -5.64 | -9.86 |
| 80% | - | - | - | - | -4.58 | -7.02 | -10.25 |
| 90% | - | - | - | - | - | -6.19 | -10.02 |
| 100% | - | - | - | - | - | - | -8.39 |

Table 9: Evaluation results of 28 models trained on different numbers of training samples and agreement rates.

$1171, 1148, 1049, 883, 672, 448, 74$. Then, we generated downsampled versions of each dataset using the found dataset sizes (where possible). This results in 28 training datasets, and we train HPSCAN for each dataset, keeping models with the best validation loss after 100 epochs with batch size 32. We then evaluate each model using an identical test dataset as used in the main paper. Performance results are reported in Table 9. The results indicate that in general, more training data improves model performance. Consequently, filtering for higher agreement rates decreases available training samples resulting in decreased evaluation results. Note, that these models did not undergo any pretraining and the full training length as in the main paper (due to limited resources available), indicated by overall worse performance results compared to the results presented in the main paper.

## 13. Vanbelle Kappa Index vs. Agreement Score - Toy Example

One crucial aspect of our proposed agreement index ($\kappa_\alpha$) is, that it measures the degree of improvement of group agreement for

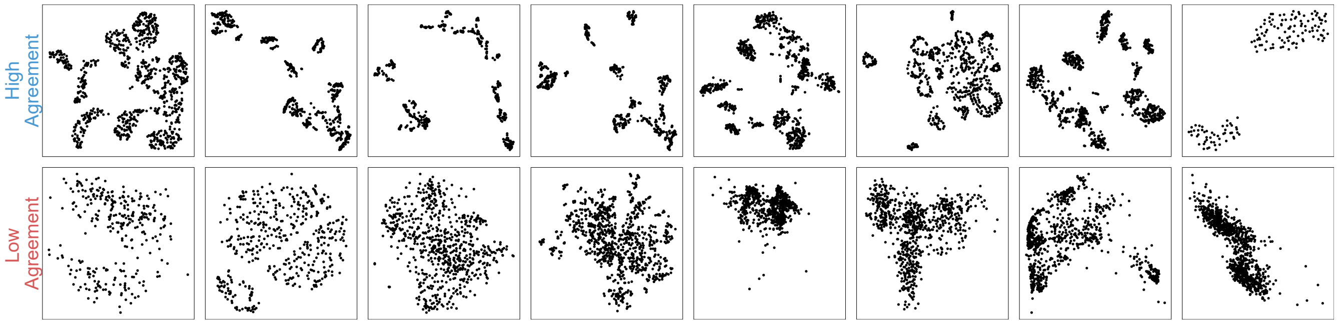


Figure 8: We apply our HPSCAN to the CLAMS dataset and estimate human agreement for all 60 stimuli. We present in the top row the eight stimuli with the highest agreement and in the bottom row the eight lowest-scored stimuli.

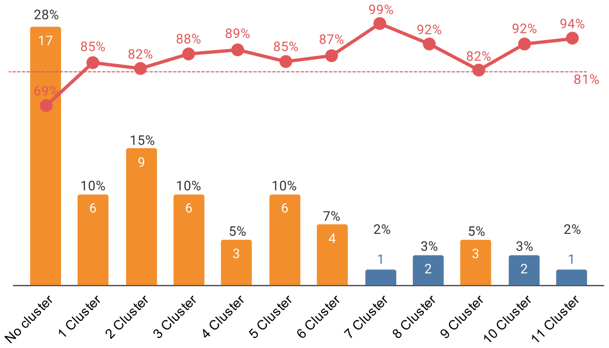


Figure 9: CLAMS consists of 60 stimuli, we show the distribution of stimuli that got annotated with a certain number of clusters. The user agreement is visualized in red for the number of clusters, respectively. Note, that for CLAMS per stimulus, 18 human raters provided clustering annotations utilizing a lasso interaction to separate clusters. The bars colored in blue represent cluster numbers with a dataset contribution below 5%.

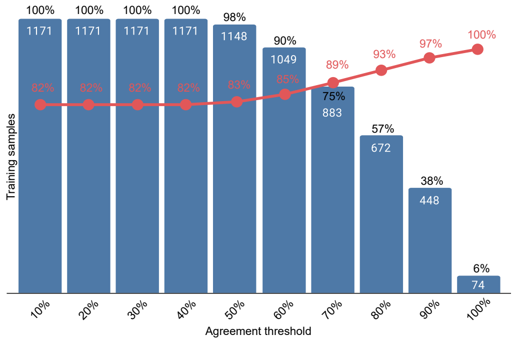


Figure 10: We filter the training dataset using different agreement thresholds $T_{agree}$, discarding training samples, where the agreement score is below such threshold. This results in different amounts of training data. For each threshold, we compute the resulting averaged agreement score for the remaining training data.

a given isolated rating. In contrast, Vanbelle Kappa Index ($\kappa_v$) is based on consensus within the group, and in the absence of variability in the classifications by the group of raters or by the isolated rater it reduces to $\kappa_v = 1.0$ for perfect agreement in group or $\kappa_v = 0.0$ else (when agreement can only be explained by pure chance [VA09]).

In this toy example, the difference of $\kappa_v$ and $\kappa_\alpha$ is demonstrated. We generated 100 random points and three scenarios, where we compute both measures based on the isolated rating and 5 group ratings, see Figure 11. In the first scenario, the isolated rating and the group ratings are identical providing annotations for a single cluster, in the second scenario we randomize the clustering of the isolated rating and keep the ratings inside the group identical (single cluster annotations). In the third scenario, the isolated rating and group rating are identical, except for one rater inside the group, where we alter half of the points to a different cluster ID (two cluster annotations). In the first two scenarios, the isolated rating gets identical $\kappa_v = 1.0$, due to the group agreement being 100%. It is clear, that for the second scenario, the isolated rating does not align well with the group ratings. Our $\kappa_\alpha$ index does indicate such poor alignment. In the third scenario, we see that $\kappa_v = 0.0$, although the isolated rating aligns well with the group, which is another shortcoming of the Vanbelle Kappa Index originating from zero variation in the isolated rating.
This toy example demonstrates the limitation of the Vanbelle Kappa Index and underlines the need for an outlier-aware rater agreement measure.

## 14. Agreement Prediction Evaluation

In Figure 12, we display visual results of HPSCAN, estimating human agreement, for three datasets. The first three rows correspond to our collected test dataset, the next three rows correspond to the SDR [SMT13] dataset, and the last three rows show results for the Data.gov dataset. We can show, that HPSCAN is able to estimate human agreement for each point individually, providing the user some insights for the provided point data and correlating human perceived clustering.

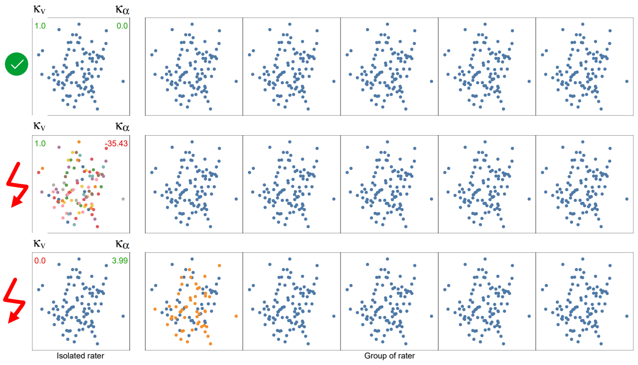


Figure 11: In this toy example the differences between Vanbelle Kappa Index ($\kappa_v$) and our proposed agreement index ($\kappa_\alpha$) is demonstrated. In the first rows, the isolated rating is identical to the group ratings resulting in $\kappa_v = 1$ and $\kappa_\alpha = 0.0$ indicating good alignment. However, in the second row, the isolated rating does not align well with the group ratings, which is not indicated by $\kappa_v = 1.0$ due to perfect group agreement. Our $\kappa_\alpha$ index does indicate such poor alignment. In the last row, we see that $\kappa_v = 0.0$, although the isolated rating aligns well with the group, which is a limitation of the Vanbelle Kappa Index originating from zero variation in the isolated rating.

## 15. Shape and Density Experiments

To investigate the sensibility of point density, we conduct an experiment where the density of points is changed by a constant factor. Therefore, each point is rescaled along all axes by the same factor altering the density of the point data without changing relative distances. We apply three scaling factors: $1.0, 0.8, 0.1$ during inference and report the results in Table 10 showing severe performance degradation for the same model and three altered versions of our test datasets for both measures $\kappa_\alpha$ and $\kappa_v$. These results indicate the sensibility of point density of HPSCAN.

In a second experiment, we investigate the shape distribution of our collected dataset by computing the covariance matrix for each cluster annotated by human raters. For each covariance matrix, the largest eigenvalues are derived and the histogram of their ratio is computed. We define the eigenvalue ratio as the quotient: $R = \frac{E_y}{E_x}$ and plot the histogram using 10 bins in Figure 13. A ratio closer to 1.0 correlates with clusters shaped like a circle, whereas ratios closer to 0.0 correlate to ellipsoid-shaped clusters. For each bin, we provide the number of clusters as well as the mean density of the clusters. Looking at the results, the majority of our collected clusters are shaped more like an ellipsoid than a circle, however, a wide variety of shapes is covered in the dataset.

| Scale factor | $\kappa_\alpha$ | $\kappa_v$ |
|---|---|---|
| 1.0 | -0.5989 | 0.6001 |
| 0.8 | -1.7912 | 0.5529 |
| 0.1 | -9.1138 | 0.1897 |

Table 10: Input points are rescaled by a constant scale factor altering the density of the points without changing relative distances. Performance degradation indicates the importance of cluster densities.

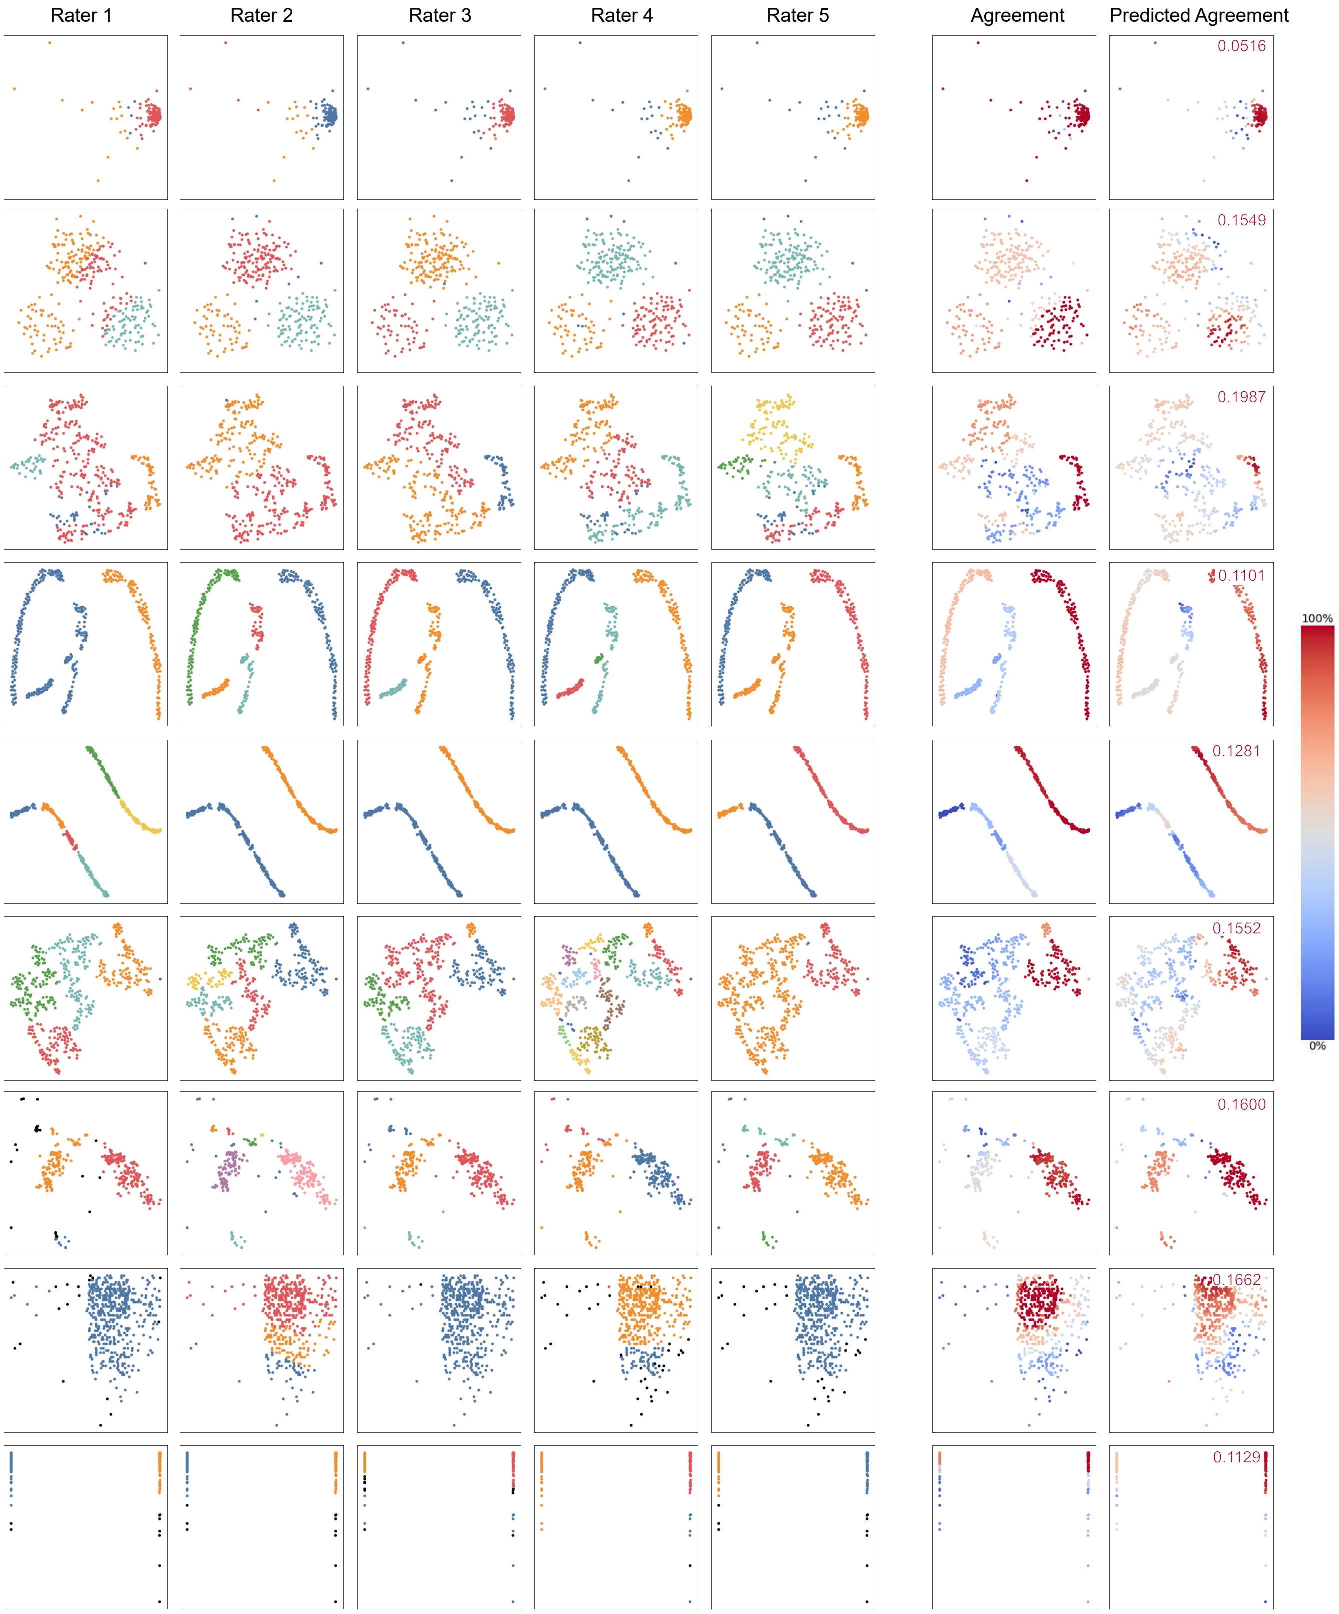


Figure 12: The first five columns display human annotations collected during our online crowdsource study. We compare annotations for six stimuli. In the sixth column, the computed agreement score per point is shown. Finally, in the last column, the prediction of HPSCAN is shown, along with the averaged absolute error overall points.

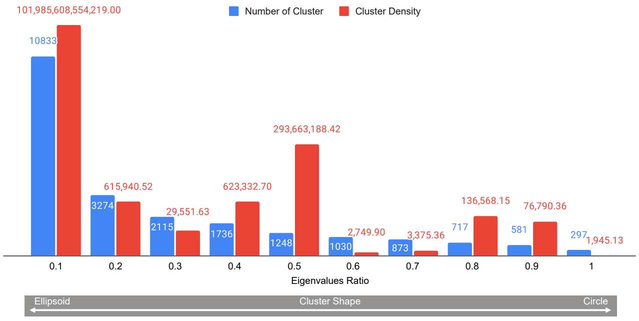


Figure 13: Histogram of eigenvalue ratio derived from the covariance matrix for each cluster. Quotients of eigenvalues closer to one correlate to circle-shaped clusters, whereas a quotient closer to zero correlates with ellipsoid-shaped clusters. Blue bars indicate the number of clusters lying inside the corresponding bin of the histogram. Red bars visualize the mean density of the clusters of the corresponding bin.
